# Supplementary material for: In-Context Code-Text Learning for Bimodal Software Engineering
Source: arXiv:2410.18107 source file (2024-10-08)
Supplement: Supplementary file 1 [file appendices.tex]

\appendices{}

\section{Datasets}
\label{appendix_datasets}

In Table~\ref{detailed_datasets}, we provide detailed information about all the datasets involved in the experiments of this work. The datasets can be downloaded using the Huggingface download interface and the corresponding repository IDs. It is worth noting that for some datasets, we only used a subset, which is indicated in the ``Remark'' column.

\begin{table*}[ht]

\centering
\captionsetup{justification=centering}
\caption{Detailed information of datasets involved in this work.}

\resizebox{.95\linewidth}{!}{
\begin{tabular}
{
>{\columncolor[HTML]{FFFFFF}}l |
>{\columncolor[HTML]{FFFFFF}}l 
>{\columncolor[HTML]{FFFFFF}}l 
>{\columncolor[HTML]{FFFFFF}}l }
\hline
{\color[HTML]{000000} \textbf{Task}}                                                     & {\color[HTML]{000000} \textbf{Dataset}}  & {\color[HTML]{000000} \textbf{Huggingface Repository ID}}                     & {\color[HTML]{000000} \textbf{Remark}}              \\ \hline
\cellcolor[HTML]{FFFFFF}{\color[HTML]{000000} }                                          & {\color[HTML]{000000} Big-Vul}           & {\color[HTML]{000000} benjis/bigvul}                                          & {\color[HTML]{000000} }                             \\
\cellcolor[HTML]{FFFFFF}{\color[HTML]{000000} }                                          & {\color[HTML]{000000} Draper}            & {\color[HTML]{000000} claudios/Draper}                                        & {\color[HTML]{000000} }                             \\
\cellcolor[HTML]{FFFFFF}{\color[HTML]{000000} }                                          & {\color[HTML]{000000} D2A}               & {\color[HTML]{000000} claudios/D2A}                                           & {\color[HTML]{000000} subset=``function''}          \\
\cellcolor[HTML]{FFFFFF}{\color[HTML]{000000} }                                          & {\color[HTML]{000000} ReVeal}            & {\color[HTML]{000000} claudios/ReVeal}                                        & {\color[HTML]{000000} }                             \\
\multirow{-5}{*}{\cellcolor[HTML]{FFFFFF}{\color[HTML]{000000} Vulnerability Detection}} & {\color[HTML]{000000} Devign}            & {\color[HTML]{000000} code\_x\_glue\_cc\_defect\_detection}                   & {\color[HTML]{000000} }                             \\ \hline
{\color[HTML]{000000} Clone Detection}                                                   & {\color[HTML]{000000} BigCloneBench}     & {\color[HTML]{000000} code\_x\_glue\_cc\_clone\_detection\_big\_clone\_bench} & {\color[HTML]{000000} }                             \\ \hline
\cellcolor[HTML]{FFFFFF}{\color[HTML]{000000} }                                          & {\color[HTML]{000000} InstructHumanEval} & {\color[HTML]{000000} codeparrot/instructhumaneval}                           & {\color[HTML]{000000} }                             \\
\multirow{-2}{*}{\cellcolor[HTML]{FFFFFF}{\color[HTML]{000000} Code Completion}}         & {\color[HTML]{000000} Safim}             & {\color[HTML]{000000} gonglinyuan/safim}                                      & {\color[HTML]{000000} }                             \\ \hline
\cellcolor[HTML]{FFFFFF}{\color[HTML]{000000} }                                          & {\color[HTML]{000000} CodeXGLUE}         & {\color[HTML]{000000} code\_x\_glue\_cc\_code\_to\_code\_trans}               & {\color[HTML]{000000} }                             \\
\multirow{-2}{*}{\cellcolor[HTML]{FFFFFF}{\color[HTML]{000000} Code Translation}}        & {\color[HTML]{000000} HumanEval-X}       & {\color[HTML]{000000} THUDM/humaneval-x}                                      & {\color[HTML]{000000} java-to-python}               \\ \hline
\cellcolor[HTML]{FFFFFF}{\color[HTML]{000000} }                                          & {\color[HTML]{000000} CodeXGLUE}         & {\color[HTML]{000000} ayeshgk/code\_x\_glue\_cc\_code\_refinement\_annotated} & {\color[HTML]{000000} }                             \\
\multirow{-2}{*}{\cellcolor[HTML]{FFFFFF}{\color[HTML]{000000} Program Repair}}          & {\color[HTML]{000000} HumanEvalPack}     & {\color[HTML]{000000} bigcode/humanevalpack}                                  & {\color[HTML]{000000} subset=``python''}            \\ \hline
\cellcolor[HTML]{FFFFFF}{\color[HTML]{000000} }                                          & {\color[HTML]{000000} CodeXGLUE}         & {\color[HTML]{000000} code\_x\_glue\_ct\_code\_to\_text}                      & {\color[HTML]{000000} subset=``java''}              \\
\cellcolor[HTML]{FFFFFF}{\color[HTML]{000000} }                                          & {\color[HTML]{000000} XLCoST}            & {\color[HTML]{000000} codeparrot/xlcost-text-to-code}                         & {\color[HTML]{000000} subset=``C++-program-level''} \\
\multirow{-3}{*}{\cellcolor[HTML]{FFFFFF}{\color[HTML]{000000} Code Summarization}}      & {\color[HTML]{000000} Funcom}            & {\color[HTML]{000000} apcl/funcom-java-long}                                  & {\color[HTML]{000000} }                             \\ \hline
\cellcolor[HTML]{FFFFFF}{\color[HTML]{000000} }                                          & {\color[HTML]{000000} APPS}              & {\color[HTML]{000000} codeparrot/apps}                                        & {\color[HTML]{000000} difficulties=``all''}         \\
\cellcolor[HTML]{FFFFFF}{\color[HTML]{000000} }                                          & {\color[HTML]{000000} MBPP}              & {\color[HTML]{000000} mbpp}                                                   & {\color[HTML]{000000} subset=``sanitized''}         \\
\cellcolor[HTML]{FFFFFF}{\color[HTML]{000000} }                                          & {\color[HTML]{000000} Mercury}           & {\color[HTML]{000000} Elfsong/Mercury}                                        & {\color[HTML]{000000} }                             \\
\cellcolor[HTML]{FFFFFF}{\color[HTML]{000000} }                                          & {\color[HTML]{000000} InstructHumanEval} & {\color[HTML]{000000} codeparrot/instructhumaneval}                           & {\color[HTML]{000000} }                             \\
\cellcolor[HTML]{FFFFFF}{\color[HTML]{000000} }                                          & {\color[HTML]{000000} StudentEval}       & {\color[HTML]{000000} wellesley-easel/StudentEval}                            & {\color[HTML]{000000} }                             \\
\cellcolor[HTML]{FFFFFF}{\color[HTML]{000000} }                                          & {\color[HTML]{000000} XLCoST}            & {\color[HTML]{000000} codeparrot/xlcost-text-to-code}                         & {\color[HTML]{000000} subset=``C++-program-level''} \\
\cellcolor[HTML]{FFFFFF}{\color[HTML]{000000} }                                          & {\color[HTML]{000000} CoNaLa}            & {\color[HTML]{000000} neulab/conala}                                          & {\color[HTML]{000000} subset=``curated''}           \\
\multirow{-8}{*}{\cellcolor[HTML]{FFFFFF}{\color[HTML]{000000} Code Generation}}         & {\color[HTML]{000000} CONCODE}           & {\color[HTML]{000000} AhmedSSoliman/CodeXGLUE-CONCODE}                        & {\color[HTML]{000000} }                             \\ \hline
\end{tabular}}

\label{detailed_datasets}
\end{table*}
